# Supplementary material for: Mode-selective vibrational control of charge transport in $\pi$-conjugated molecular materials
Source: arXiv:1503.00777 ancillary file (2015-03-02)
Supplement: Supplementary file 1 [file Suppl-Info_VibControl_Arxiv.pdf]

# Supplementary Information for

## Mode-selective vibrational control of charge transport in $\pi$ -conjugated molecular materials

Artem A. Bakulin<sup>1,5\*+</sup>, Robert Lovrincic<sup>2,4\*</sup>, Yu Xi<sup>2\*</sup>, Oleg Selig<sup>1</sup>, Huib J. Bakker<sup>1</sup>,  
Yves L.A. Rezus<sup>1</sup>, Pabitra K. Nayak<sup>2#</sup>, Alexandr Fonari<sup>3</sup>, Veaceslav Coropceanu<sup>3</sup>,  
Jean-Luc Brédas,<sup>3,6</sup> and David Cahen<sup>2+</sup>

<sup>1</sup> FOM Institute AMOLF, Science Park 104, 1098 XG Amsterdam, The Netherlands

<sup>2</sup> Weizmann Institute of Science, Rehovot 76100, Israel

<sup>3</sup> School of Chemistry and Biochemistry & Center for Organic Photonics and Electronics,  
Georgia Institute of Technology, 901 Atlantic Drive NW, Atlanta, GA 30332-0400, USA

<sup>4</sup> Braunschweig University, Innovationlab, Speyerer Straße 4, Heidelberg 69115, Germany

<sup>5</sup> Cavendish Laboratory, University of Cambridge, JJ Thomson Avenue, Cambridge CB30HE, UK

<sup>6</sup> Solar & Photovoltaics Engineering Research Center, , King Abdullah University of Science and  
Technology, Thuwal 23955-6900, Kingdom of Saudi Arabia

\* Equal contribution

+ Corresponding authors: [aab58@cam.ac.uk](mailto:aab58@cam.ac.uk); [david.cahen@weizmann.ac.il](mailto:david.cahen@weizmann.ac.il)

# Current address: Clarendon Laboratory, University of Oxford, Oxford, UK, OX1 3PU

### Contents:

1. Details of theoretical modeling
2. Device IV characterization
3. Angle-dependent IR absorption
4. Experimental details
5. Time-domain Fourier filtering

## 1. Details of theoretical calculations

Geometry optimizations of the crystal structure of the triclinic pentacene polymorph proposed by Campbell<sup>1</sup> were performed at the PBE0/6-31G level of theory. During the optimization, the unit-cell parameters were kept fixed at the experimental values. A uniform 8x6x4 Monkhorst-Pack k-point grid was employed. The  $\Gamma$ -point phonons (lattice vibrations) within the harmonic approximation and the IR intensities were obtained via a coupled perturbed Hartree-Fock (CPHF) approach. These calculations were carried out with the CRYSTAL14 package.<sup>2,3</sup> Since there are two independent molecules in the unit cell of the pentacene crystal, all molecular vibration modes are two-fold (quasi)degenerate. All lattice vibrations in the region of interest can be visualized on the Internet [<http://afonari.com/pentacene-vibrations/>].

Transfer integrals (electronic couplings) for holes were calculated using a fragment orbital approach based on the unperturbed highest occupied molecular orbitals (HOMOs) of the individual neutral molecules extracted from the optimized crystal geometry.<sup>4</sup> The nonlocal hole-phonon coupling constants ( $\nu$ ) come from the modulation of the transfer integrals by lattice vibrations. The coupling constants can be computed by expanding the electronic couplings into Taylor series of the phonon eigenvectors:  $t = t_0 + \sum_j \nu_j Q_j$ . Here,  $t_0$  is the electronic coupling at the crystal equilibrium geometry;  $Q_j$  is the normal-mode coordinate of mode  $j$ ;  $\nu_j$  is the linear nonlocal electron-phonon coupling constant. In practice, the coupling constants are calculated by distorting the crystal along all normal-mode coordinates with positive and negative steps and then computing numerically the related derivatives of the transfer integrals for each vibrational mode.

All the calculations for the isolated neutral and positively charged molecules were performed at the PBE0/6-31G level of theory using the Gaussian package.<sup>5</sup> The normal modes of the neutral ( $Q_n$ ) and cation ( $Q_c$ ) states are related to each other via a multidimensional rotation (Duschinsky) matrix (Table S2).<sup>6</sup> The Duschinsky matrix was computed with the DUSHIN code.<sup>7</sup> The calculated frequencies for both isolated molecule and crystal were scaled by 0.95 (Table S1).<sup>8</sup>

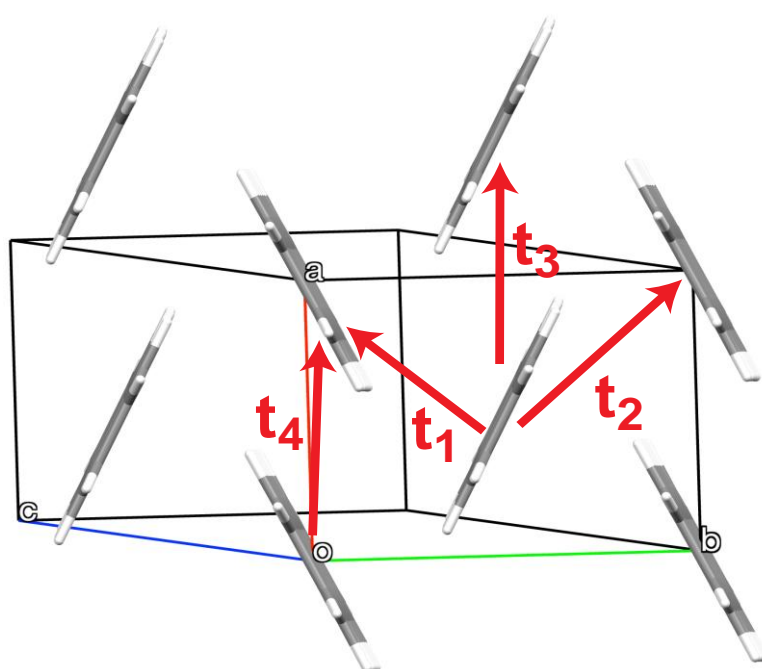

*Figure S1. Crystal packing of pentacene. The largest hole charge transfer integrals are shown in red:  $t_1 = 75$  meV,  $t_2 = 32$  meV,  $t_3 = 20$  meV,  $t_4 = 6$  meV. Note that IR-active modes do not modulate transfer integrals  $t_3$ ,  $t_4$ .<sup>9</sup>*

Table S1. Frequencies, IR intensities, and nonlocal hole-phonon couplings for pentacene.

| Crystal                 |            |                      |                      | Neutral molecule        |            | Charged molecule        |            |
|-------------------------|------------|----------------------|----------------------|-------------------------|------------|-------------------------|------------|
| Freq., cm <sup>-1</sup> | IR, km/mol | v <sub>1</sub> , meV | v <sub>2</sub> , meV | Freq., cm <sup>-1</sup> | IR, km/mol | Freq., cm <sup>-1</sup> | IR, km/mol |
| 970.13                  | 77.04      | 0.21                 | 0.07                 | 913.29                  | 129.07     | 939.34                  | 93.61      |
| 970.63                  | 36.75      | 0.14                 | 0.07                 | 958.03                  | 17.55      | 977.01                  | 21.64      |
| 992.53                  | 21.65      | 0.43                 | 0.43                 | 995.98                  | 5.69       | 1013.59                 | 0.09       |
| 994.90                  | 0.09       | 0.79                 | 2.86                 | 1113.81                 | 7.96       | 1116.32                 | 3.92       |
| 997.79                  | 28.24      | 0.00                 | 0.79                 | 1133.71                 | 4.91       | 1166.38                 | 28.84      |
| 1001.41                 | 2.51       | 0.14                 | 0.21                 | 1163.09                 | 0.26       | 1176.69                 | 198.32     |
| 1110.80                 | 36.33      | 0.07                 | 0.00                 | 1186.55                 | 3.62       | 1188.85                 | 2.75       |
| 1113.74                 | 16.09      | 0.07                 | 0.14                 | 1228.96                 | 1.66       | 1235.58                 | 131.09     |
| 1137.16                 | 4.55       | 0.29                 | 0.43                 | 1268.43                 | 0.01       | 1273.24                 | 2.23       |
| 1138.36                 | 5.14       | 0.07                 | 0.93                 | 1284.67                 | 24.38      | 1288.99                 | 41.72      |
| 1158.93                 | 5.68       | 0.07                 | 0.29                 | 1335.15                 | 13.96      | 1336.43                 | 6.29       |
| 1164.37                 | 36.81      | 0.07                 | 0.07                 | 1342.13                 | 2.51       | 1380.13                 | 653.83     |
| 1187.31                 | 2.96       | 0.29                 | 0.07                 | 1405.31                 | 2.50       | 1400.18                 | 839.40     |
| 1190.04                 | 41.10      | 0.07                 | 0.07                 | 1410.59                 | 0.87       | 1415.26                 | 148.93     |
| 1228.30                 | 14.87      | 0.29                 | 1.14                 | 1440.56                 | 0.86       | 1438.87                 | 20.08      |
| 1230.19                 | 1.28       | 0.50                 | 1.00                 | 1442.49                 | 1.27       | 1444.38                 | 6.94       |
| 1272.59                 | 1.01       | 0.29                 | 0.14                 | 1508.64                 | 2.99       | 1488.77                 | 502.01     |
| 1274.71                 | 4.63       | 0.29                 | 0.14                 | 1544.89                 | 3.08       | 1530.31                 | 292.10     |
| 1283.62                 | 81.01      | 0.43                 | 0.43                 | 1601.88                 | 1.56       | 1578.82                 | 3.89       |
| 1287.69                 | 36.16      | 0.43                 | 0.57                 | 1637.32                 | 10.38      | 1598.20                 | 20.13      |
| 1336.47                 | 4.64       | 0.07                 | 0.43                 |                         |            |                         |            |
| 1338.68                 | 15.22      | 0.21                 | 0.50                 |                         |            |                         |            |
| 1340.40                 | 15.86      | 0.86                 | 0.29                 |                         |            |                         |            |
| 1342.41                 | 16.93      | 0.43                 | 0.50                 |                         |            |                         |            |
| 1404.86                 | 4.47       | 0.07                 | 0.00                 |                         |            |                         |            |
| 1406.01                 | 4.80       | 0.93                 | 0.79                 |                         |            |                         |            |
| 1413.53                 | 0.14       | 0.21                 | 0.64                 |                         |            |                         |            |
| 1414.51                 | 0.63       | 0.36                 | 0.43                 |                         |            |                         |            |
| 1437.36                 | 9.19       | 0.36                 | 0.07                 |                         |            |                         |            |
| 1438.79                 | 21.27      | 0.86                 | 2.14                 |                         |            |                         |            |
| 1438.95                 | 33.94      | 0.36                 | 0.79                 |                         |            |                         |            |
| 1440.53                 | 12.79      | 0.64                 | 2.07                 |                         |            |                         |            |
| 1503.93                 | 6.16       | 1.21                 | 2.00                 |                         |            |                         |            |
| 1504.28                 | 23.99      | 1.86                 | 1.21                 |                         |            |                         |            |
| 1540.27                 | 34.73      | 1.71                 | 2.43                 |                         |            |                         |            |
| 1541.25                 | 14.26      | 0.50                 | 1.57                 |                         |            |                         |            |
| 1594.79                 | 12.50      | 0.64                 | 1.36                 |                         |            |                         |            |
| 1595.31                 | 3.98       | 0.21                 | 0.93                 |                         |            |                         |            |
| 1632.15                 | 43.92      | 4.00                 | 0.93                 |                         |            |                         |            |
| 1633.17                 | 16.82      | 1.21                 | 0.64                 |                         |            |                         |            |

Table S2. Correspondence between frequencies of cation and neutral molecule based on the projections of the normal coordinates of the charged molecule onto the neutral molecule normal coordinates. Largest coefficients of Duschinsky matrices are also listed.

| Cation freq., cm <sup>-1</sup> | Neutral freq., cm <sup>-1</sup> | %    |
|--------------------------------|---------------------------------|------|
| 939.34                         | 913.29                          | 99.6 |
| 977.01                         | 958.03                          | 99.7 |
| 1013.59                        | 995.98                          | 99.2 |
| 1116.32                        | 1113.81                         | 98.8 |
| 1166.38                        | 1133.71                         | 73.8 |
|                                | 1163.09                         | 22.3 |
| 1176.69                        | 1133.71                         | 21.5 |
|                                | 1163.09                         | 76.7 |
| 1188.85                        | 1186.55                         | 98.1 |
| 1235.58                        | 1228.96                         | 96.7 |
| 1273.24                        | 1268.43                         | 93.8 |
| 1288.99                        | 1284.67                         | 95.6 |
| 1336.43                        | 1342.13                         | 96.1 |
| 1380.13                        | 1335.15                         | 18.5 |
|                                | 1405.31                         | 52   |
|                                | 1544.89                         | 10.1 |
| 1400.18                        | 1335.15                         | 68.5 |
|                                | 1410.59                         | 11.5 |
| 1415.26                        | 1405.31                         | 26.6 |
|                                | 1410.59                         | 56.8 |
| 1438.87                        | 1410.59                         | 88.6 |
| 1444.38                        | 1442.49                         | 97.2 |
| 1488.77                        | 1508.64                         | 77.9 |
| 1530.31                        | 1544.89                         | 77.8 |
| 1578.82                        | 1601.88                         | 88.5 |
|                                | 1637.32                         | 10.1 |
| 1598.20                        | 1601.88                         | 10.2 |
|                                | 1637.32                         | 88.9 |

**1284 cm<sup>-1</sup>**

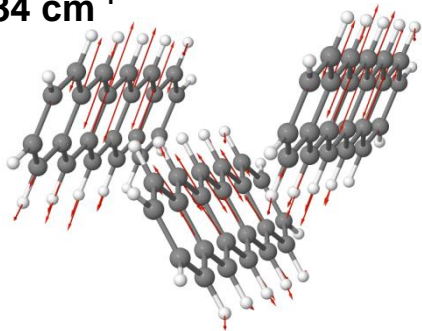

**1345 cm<sup>-1</sup>**

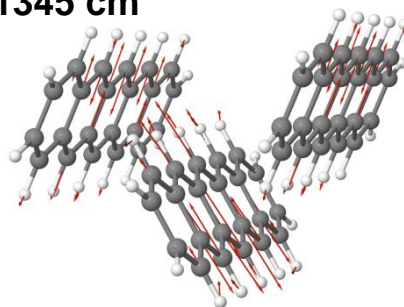

**1439 cm<sup>-1</sup>**

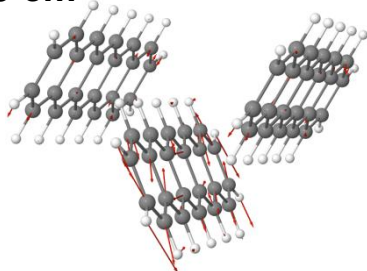

**1504 cm<sup>-1</sup>**

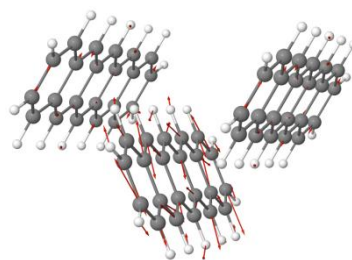

**1540 cm<sup>-1</sup>**

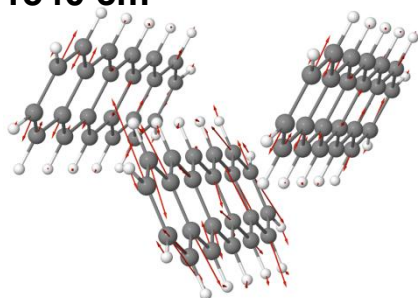

**1632 cm<sup>-1</sup>**

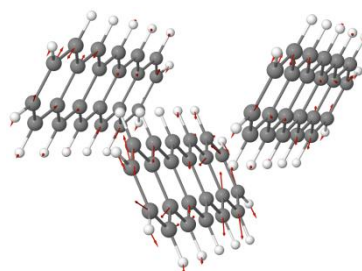

*Figure S2. Eigendisplacements corresponding to the vibrational modes addressed in the study.*

## 2. Device IV characterization

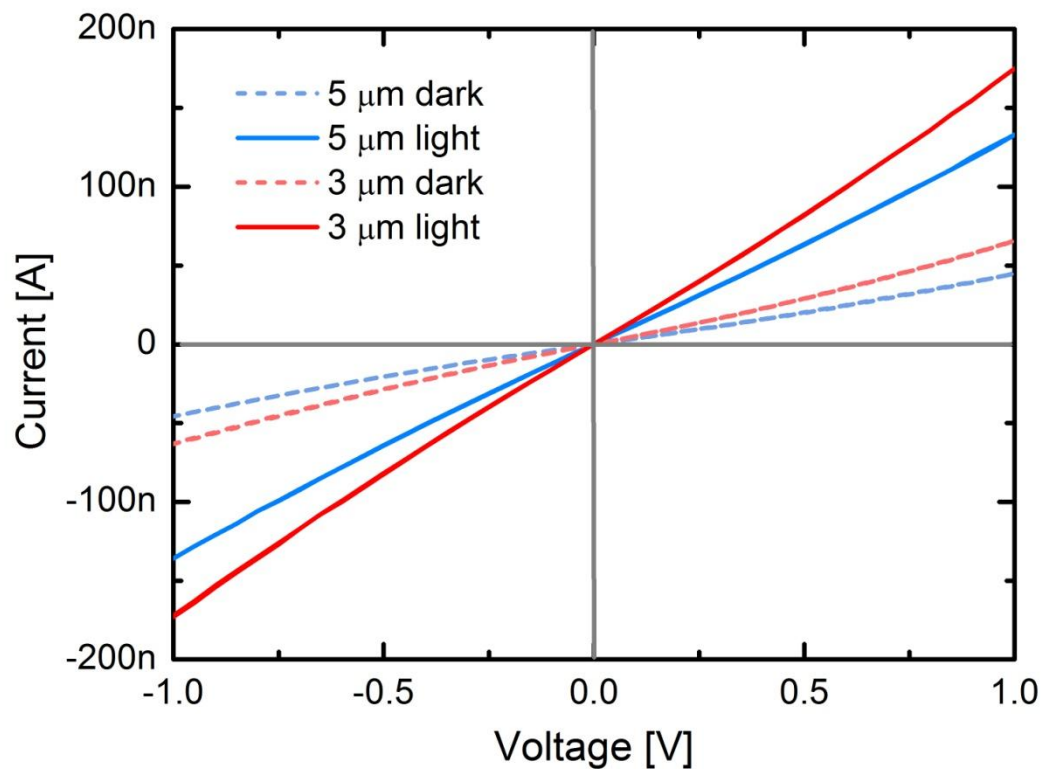

Figure S3. Typical I-V characteristics of the studied pentacene/ $C_{60}$  devices with 3 and 5  $\mu m$  electrode spacing; visible-light illumination was about  $10 \text{ mW/cm}^2$  provided by a halogen lamp.

### 3. Angle-dependent absorption in the active layer

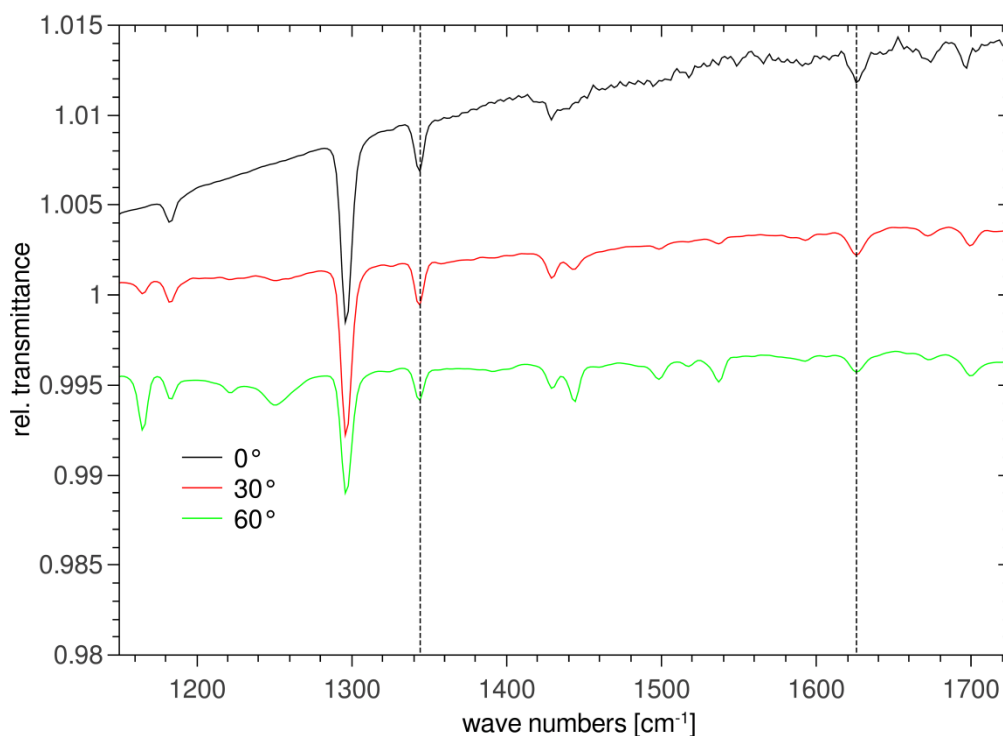

*Figure S4 Relative transmittance spectra of a pentacene/C<sub>60</sub> (70nm/15nm) film on Si at different angles of incidence (with respect to the surface normal). The absorptions of the two modes marked with dashed lines exhibit very similar angle dependence, but strongly differ in PPP coupling (see Figure 3b).*

Figure S4 shows the angle dependence of the IR absorption in the fingerprint region for a pentacene/C<sub>60</sub> layer (thicknesses identical to those used in device) on Si (measured with p-polarized light). A strong increase in peak height with increasing angle points to a transition with dipole moment perpendicular to the surface, whereas a decrease points to a dipole moment parallel to the surface. The two marked peaks at 1345 cm<sup>-1</sup> and 1630 cm<sup>-1</sup> behave similar under tilt (indicating similar orientations for the transition dipoles), but exhibit very different PPP couplings (~3 times stronger for the vibration at 1630 cm<sup>-1</sup>). We conclude from this observation that the non-scaling of the PPP response with IR absorption is not merely an effect of different orientation of the dipoles, but does reflect the different coupling strengths between charge carriers and vibrations.

## 4. Experimental details

### Materials and devices:

The gold electrodes for the phototransistor were fabricated on a SiO<sub>2</sub> substrate by a standard microfabrication technique with sequential processes of photolithography, metal evaporation, and lift-off. 70 nm pentacene and 15 nm C<sub>60</sub> film were thermo evaporated without substrate heating at rate around 0.5 Å/s. Sample were kept in N<sub>2</sub> atmosphere from fabrication until the ultrafast measurements. Ultrafast experiments were performed inside a N<sub>2</sub> flow compartment. Angle dependent IR absorption spectroscopy was done using Nocolet 6700 multi angle FT IR spectrometer with a shuttle sample holder that can change the angle of the substrate relative to the IR beam. The sample is a 70-nm thick pentacene film that was thermo evaporated on a double side polished silica substrate with native thin SiO<sub>2</sub> layer. Like for device fabrication, the evaporation was done without substrate heating. IV curves were measured using commercial source-measurement unit (Agilent B2900A) and a halogen lamp for light/dark measurements.

### Ultrafast experiments:

Pump and push pulses were generated by using the output of a 1-kHz repetition rate femtosecond regenerative amplifier (800 nm, 35 fs, 4 mJ/pulse), which by employing a beam splitter (3:1) pumped a pair of optical parametric amplifiers (TOPAS). To generate the pump pulse the ‘signal’ output of one of the TOPAS was frequency doubled in BBO crystal. For IR-push generation the signal and idler pulses from the other TOPAS were difference-frequency mixed in a AgGaS<sub>2</sub> crystal. This provided a femtosecond (100 fs, ~20 μJ) infrared pulse centered at 1360 or 1550 cm<sup>-1</sup>. After this IR light entered a Mach-Zehnder interferometer a pair of collinear push pulses was produced with the spectrum:<sup>10</sup>  $I_{pp}(\omega) = I(\omega)(2 + 2\cos(\omega\tau))$  where  $I(\omega)$  is the spectrum of a single push pulse;  $\tau$  is the delay between the two pulses. The interferometer was controlled using a reference beam from a He-Ne laser following the path of the IR beam. Both pump (<10nJ) and push (~1μJ) pulses were focused on the device using a R=15 cm spherical gold mirror. The device was biased (~5V) using a battery voltage source. Current modulation  $dI$  was detected using a lock-in amplifier (Stanford Research 510) in the current mode locked to the mechanical modulator (370 Hz) in the push beam. PPP interferogram was recorded as a function of the delay between the two push pulses  $\tau$ . The Fourier transformation of this time variable yielded the pump-frequency axis in the PPP spectrum. All measurements were performed at room temperature and N<sub>2</sub> flow atmosphere.

## 5. Time domain Fourier filtering

The experimentally detected response was typically a superposition of vibrational response (narrow lines in the frequency domain) as well as electronic and field-induced tunneling responses (broad bands in the frequency domain).<sup>11,12</sup> To extract the vibrational signals from the total response we have developed a time-domain filtering procedure which effectively suppressed all the broad feature in PPP spectra.

First the interferometric delay  $\tau=0$  is determined using the signal in the reference arm of Mach-Zehnder interferometer. The  $dJ/J(\tau)$  interferogram is then ‘zeroed’ - shifted accordingly along the interferometric time axis. After this the interferogram is multiplied by the following filtering function:

$$f(\tau) = 1 - [0.95 \exp(-\tau^2/2\Delta\tau^2)]$$

Where,  $\Delta\tau$  is a phenomenological filtering parameter, typically comparable to the inversed bandwidth of IR push spectrum ( $\Delta\tau \sim 200$  fs). Such filtering leads to the suppression of the central part of the interferogram and to the corresponding exclusion of broad features from the Fourier Transform (FT) PPP spectrum. At the same time, such filtering does not alter the phase information contained in the data which makes it more stable compared to any other filtering procedure we employed.

The robustness of time-domain filtering is illustrated in the figure 5S. A model superposition spectrum of narrow and broad spectral features (Fig. 5Sa) is used to generate a model interferogram containing both ‘electronic’ and ‘vibrational’ responses (Fig. 5Sb, black line). After the filter (Fig. 5Sb, blue line) being applied, a new interferogram (Fig. 5Sb, purple line) is produced. This new interferogram contains exclusively vibrational response which is only slightly distorted compared to the input data (Fig. 5Sc).

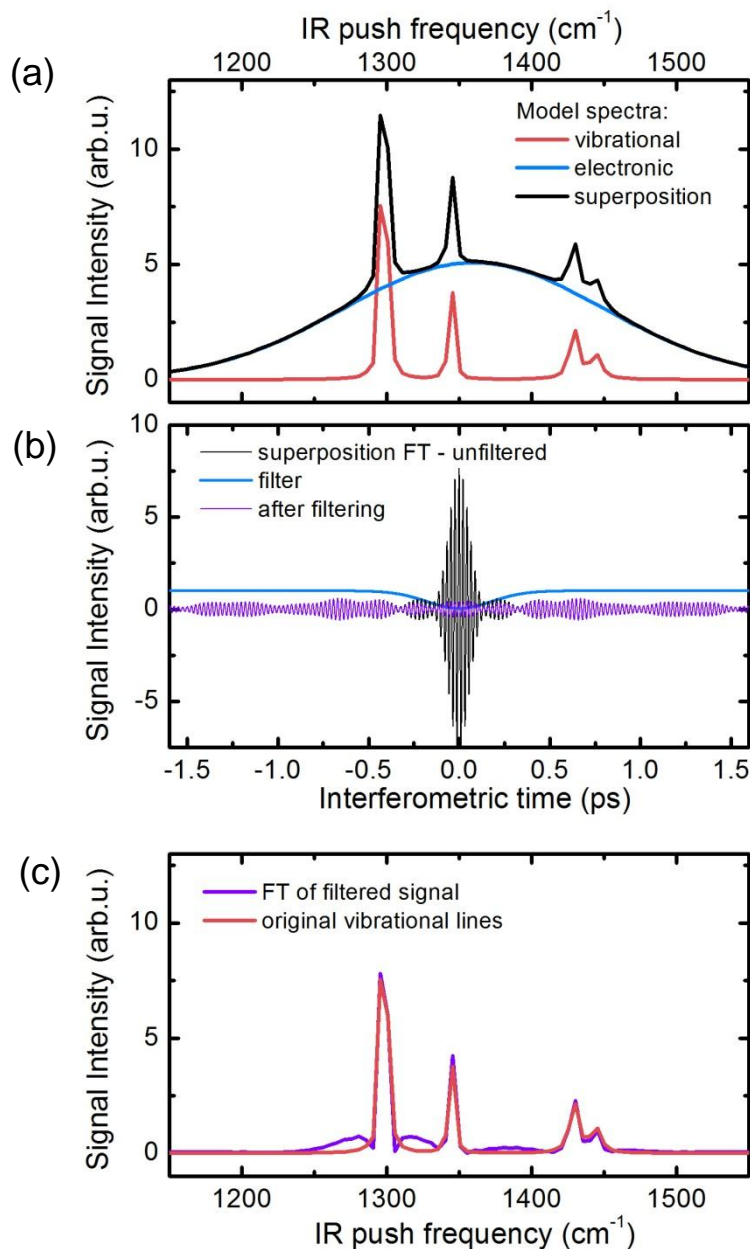

Figure S5. Illustration and accuracy check for the time-domain filtering procedure. (a) Red and blue lines show the 'model'  $dJ/J$  responses due to push-induced vibrational and electronic transitions. Black curve is a superposition of responses typically observed in the experiments. (b) Black line shows time-domain representation of the superposition curve from figure a; this represents typical experimentally observed interferogram. Blue line shows a Gaussian time-domain filter. Purple line shows a filtered interferogram. (c) Purple line is a PPP spectrum obtained by FT of filtered interferogram. It is almost identical to the vibrational part of the input signal (a).

## References:

- 1 Campbell, R. B., Robertson, J. M. & Trotter, J. The crystal structure of hexacene, and a revision of the crystallographic data for tetracene. *Acta Crystallographica* **15**, 289-290, doi:doi:10.1107/S0365110X62000699 (1962).
- 2 Maschio, L., Kirtman, B., Orlando, R. & R  rat, M. Ab initio analytical infrared intensities for periodic systems through a coupled perturbed Hartree-Fock/Kohn-Sham method. *The Journal of Chemical Physics* **137**, -, doi:doi:<http://dx.doi.org/10.1063/1.4767438> (2012).
- 3 Dovesi, R. *et al.* CRYSTAL14: A program for the ab initio investigation of crystalline solids. *International Journal of Quantum Chemistry* **114**, 1287-1317, doi:10.1002/qua.24658 (2014).
- 4 Valeev, E. F., Coropceanu, V., da Silva Filho, D. A., Salman, S. & Br  das, J.-L. Effect of Electronic Polarization on Charge-Transport Parameters in Molecular Organic Semiconductors. *Journal of the American Chemical Society* **128**, 9882-9886, doi:10.1021/ja061827h (2006).
- 5 Gaussian 09 (Gaussian, Inc., Wallingford, CT, USA, 2009).
- 6 Duschinsky, F. *URSS Acta Physicochim* **7**, 551 (1937).
- 7 Reimers, J. R. A practical method for the use of curvilinear coordinates in calculations of normal-mode-projected displacements and Duschinsky rotation matrices for large molecules. *The Journal of Chemical Physics* **115**, 9103-9109, doi:doi:<http://dx.doi.org/10.1063/1.1412875> (2001).
- 8 Langhoff, S. R. Theoretical Infrared Spectra for Polycyclic Aromatic Hydrocarbon Neutrals, Cations, and Anions. *The Journal of Physical Chemistry* **100**, 2819-2841, doi:10.1021/jp952074g (1996).
- 9 Girlando, A. *et al.* Interaction of charge carriers with lattice and molecular phonons in crystalline pentacene. *Journal of Chemical Physics* **135** (2011).
- 10 Helbing, J. & Hamm, P. Compact implementation of Fourier transform two-dimensional IR spectroscopy without phase ambiguity. *Journal of the Optical Society of America B* **28**, 171-178, doi:10.1364/josab.28.000171 (2011).
- 11 Bakulin, A. A. *et al.* The Role of Driving Energy and Delocalized States for Charge Separation in Organic Semiconductors. *Science* **335**, 1340-1344, doi:10.1126/science.1217745 (2012).
- 12 Schiffrin, A. *et al.* Optical-field-induced current in dielectrics. *Nature* **493**, 70-74, doi:<http://www.nature.com/nature/journal/v493/n7430/abs/nature11567.html#supplementary-information> (2013).
